# Supplementary material for: CellPath-Bench: A Multidimensional Benchmark for Whole-Slide Cellular Representations in Pathology Foundation Models
Source: arXiv:2608.21060 source file (2026-08-21)
Supplement: Supplementary file 1 [file Celltype_markers_copy.tex]

% Auto-generated from 03_72_celltype_markers_audited.xlsx
% Retains 68 biological cell types and excludes four state/QC labels:
% necrotic_cell, apoptotic_cell, mitotic_cell, and uncertain_cell.
%
% Required packages in the main preamble:
% \usepackage{booktabs,longtable,array,ragged2e}
% Add the bibliography file with:
% \bibliography{references_68_celltype_markers}
%
\clearpage

\begingroup
\scriptsize
\setlength{\tabcolsep}{2.1pt}
\renewcommand{\arraystretch}{1.06}
\setlength{\LTleft}{0pt}
\setlength{\LTright}{0pt}
\LTcapwidth=\textwidth
\makeatletter
\renewcommand{\fnum@table}{\normalsize\tablename~\thetable}% caption label at normal size
\makeatother
\begin{longtable}{@{}
>{\centering\arraybackslash}p{0.025\linewidth}
>{\raggedright\arraybackslash}p{0.140\linewidth}
>{\raggedright\arraybackslash}p{0.180\linewidth}
>{\raggedright\arraybackslash}p{0.160\linewidth}
>{\raggedright\arraybackslash}p{0.150\linewidth}
>{\raggedright\arraybackslash}p{0.125\linewidth}
>{\raggedright\arraybackslash}p{0.135\linewidth}
@{}}
\caption{\normalsize
\textbf{Marker definitions for the 68 biological cell types retained in the annotation taxonomy.}
\textbf{Coarse} and \textbf{Fine} denote the three-class and nine-class taxonomies, respectively, and
the \textbf{Cell type} labels follow the harmonized 68-cell-type ontology.
\textbf{Primary} and \textbf{secondary} markers are reproduced from the curated marker table.
Four state or quality-control labels (necrotic, apoptotic, mitotic, and uncertain cells) are excluded.
}
\label{tab:celltype_markers_68}\\
\toprule
\textbf{No.} & \textbf{Coarse} & \textbf{Fine} & \textbf{Cell type} &
\textbf{Primary markers} & \textbf{Secondary markers} & \textbf{Refs.} \\
\midrule
\endfirsthead
\multicolumn{7}{l}{\tablename~\thetable\ (continued)}\\
\toprule
\textbf{No.} & \textbf{Coarse} & \textbf{Fine} & \textbf{Cell type} &
\textbf{Primary markers} & \textbf{Secondary markers} & \textbf{Refs.} \\
\midrule
\endhead
\midrule
\multicolumn{7}{r}{Continued on next page}\\
\endfoot
\bottomrule
\endlastfoot
1 & Epithelial/\allowbreak{}Tumor & Neoplastic & Tumor epithelial general & EPCAM, KRT18, KRT8 & MKI67, TOP2A, PCNA & \cite{pmid42066759,pmid41895279,pmid41544627} \\
2 & Epithelial/\allowbreak{}Tumor & Neoplastic & Adenocarcinoma cell & CK7, CK20, MUC1, CDX2 & CEA, EMA & \cite{pmid42066759,pmid41966692,pmid40345189} \\
3 & Epithelial/\allowbreak{}Tumor & Neoplastic & Squamous carcinoma cell & CK5/6, p63, p40 & CK14, DSG3 & \cite{pmid41073785,pmid41529665,pmid41961948} \\
4 & Epithelial/\allowbreak{}Tumor & Neoplastic & Neuroendocrine tumor cell & SYN, CgA, INSM1 & -- & \cite{pmid39724105,pmid39983726,pmid41501470} \\
5 & Epithelial/\allowbreak{}Tumor & Neoplastic & Undifferentiated tumor cell & Vimentin$\pm$, CK$\pm$ & -- & \cite{pmid39548577} \\
6 & Epithelial/\allowbreak{}Tumor & Neoplastic & Clear cell carcinoma & CA9, PAX8, HIF1A & VEGFA, VHL & \cite{pmid40345189,pmid41997105} \\
7 & Epithelial/\allowbreak{}Tumor & Neoplastic & Melanoma cell & MLANA, SOX10, PMEL & MITF, S100B, TYR & \cite{pmid41038164,pmid41100131,pmid38759655} \\
8 & Epithelial/\allowbreak{}Tumor & Non-neoplastic epithelial/\allowbreak{}parenchymal & Normal epithelial general & EPCAM, KRT18 & CDH1, KRT8 & \cite{pmid42185888,pmid42204317,pmid42203883} \\
9 & Epithelial/\allowbreak{}Tumor & Non-neoplastic epithelial/\allowbreak{}parenchymal & Hepatocyte & ALB, HNF4A, CYP3A4 & ASGR1, AFP & \cite{pmid41986723,pmid41435820,pmid33357445} \\
10 & Epithelial/\allowbreak{}Tumor & Non-neoplastic epithelial/\allowbreak{}parenchymal & Cholangiocyte & KRT19, SOX9, KRT7 & -- & \cite{pmid41963321,pmid42020743,pmid41202811} \\
11 & Epithelial/\allowbreak{}Tumor & Non-neoplastic epithelial/\allowbreak{}parenchymal & AT2 cell & SFTPC, SFTPB, NKX2-1 & ABCA3, LAMP3 & \cite{pmid42020743,pmid41202811,pmid41578022} \\
12 & Epithelial/\allowbreak{}Tumor & Non-neoplastic epithelial/\allowbreak{}parenchymal & Club cell & SCGB1A1, CYP2F1 & -- & \cite{pmid41578022,pmid40399607,pmid42103706} \\
13 & Epithelial/\allowbreak{}Tumor & Non-neoplastic epithelial/\allowbreak{}parenchymal & Ciliated epithelial & FOXJ1, DNAH5 & -- & \cite{pmid41578022,pmid42240739,pmid42103706} \\
14 & Epithelial/\allowbreak{}Tumor & Non-neoplastic epithelial/\allowbreak{}parenchymal & Goblet cell & MUC2, TFF3, FCGBP & CLCA1, SPDEF & \cite{pmid42020743,pmid41202811} \\
15 & Epithelial/\allowbreak{}Tumor & Non-neoplastic epithelial/\allowbreak{}parenchymal & Paneth cell & LYZ, DEFA5, REG3A & -- & \cite{pmid42020743,pmid41202811} \\
16 & Epithelial/\allowbreak{}Tumor & Non-neoplastic epithelial/\allowbreak{}parenchymal & Enterocyte & FABP2, VIL1, SI & -- & \cite{pmid42097141,pmid42154581,pmid42084500} \\
17 & Epithelial/\allowbreak{}Tumor & Non-neoplastic epithelial/\allowbreak{}parenchymal & Acinar cell & AMY2A, PRSS1, CPA1 & CELA3A, PNLIP & \cite{pmid41495736,pmid41997105,pmid41758082} \\
18 & Epithelial/\allowbreak{}Tumor & Non-neoplastic epithelial/\allowbreak{}parenchymal & Islet cell & INS, GCG, SST & -- & \cite{pmid40269162,pmid42066759,pmid41895277} \\
19 & Epithelial/\allowbreak{}Tumor & Non-neoplastic epithelial/\allowbreak{}parenchymal & Ductal cell & KRT19, SOX9, MUC1 & -- & \cite{pmid42066759,pmid42119923,pmid41593194} \\
20 & Epithelial/\allowbreak{}Tumor & Non-neoplastic epithelial/\allowbreak{}parenchymal & Tubular epithelial cell & AQP1 (PCT), UMOD (TAL) & -- & \cite{pmid41241671,pmid42091869} \\
21 & Epithelial/\allowbreak{}Tumor & Non-neoplastic epithelial/\allowbreak{}parenchymal & Podocyte & NPHS1, NPHS2, WT1 & -- & \cite{pmid42056516,pmid42151416,pmid40169792} \\
22 & Epithelial/\allowbreak{}Tumor & Non-neoplastic epithelial/\allowbreak{}parenchymal & Keratinocyte & KRT14, KRT10, IVL & -- & \cite{pmid42204317,pmid40670711,pmid41872488} \\
23 & Epithelial/\allowbreak{}Tumor & Non-neoplastic epithelial/\allowbreak{}parenchymal & Melanocyte & MLANA, PMEL, MITF & -- & \cite{pmid41872488,pmid42151416,pmid41997105} \\
24 & Other/\allowbreak{}QC & Other cells & Astrocyte & GFAP, AQP4, S100B & -- & \cite{pmid42151416,pmid42135512,pmid41844611} \\
25 & Other/\allowbreak{}QC & Other cells & Neuron & RBFOX3, MAP2, SYP & -- & \cite{pmid42199117,pmid41803120,pmid41713412} \\
26 & Other/\allowbreak{}QC & Other cells & Oligodendrocyte & OLIG2, MBP, MOG & -- & \cite{pmid41167189,pmid42151483,pmid41844611} \\
27 & Epithelial/\allowbreak{}Tumor & Non-neoplastic epithelial/\allowbreak{}parenchymal & Fallopian tube epithelial & PAX8, WT1 & -- & \cite{pmid41407855,pmid39704522,pmid42010243} \\
28 & Epithelial/\allowbreak{}Tumor & Non-neoplastic epithelial/\allowbreak{}parenchymal & Ovarian surface epithelial & KRT7, PAX8, MUC16 & -- & \cite{pmid39704522,pmid41661089,pmid41407855} \\
29 & Epithelial/\allowbreak{}Tumor & Non-neoplastic epithelial/\allowbreak{}parenchymal & Granulosa cell & FOXL2, INHA, AMH & -- & \cite{pmid41407855,pmid41435820,pmid39704522} \\
30 & Immune/\allowbreak{}Inflammatory & Lymphocyte & CD8 T cell & CD8A, CD3E, GZMB & PRF1, IFNG, NKG7 & \cite{pmid42056516,pmid41986723,pmid41951740} \\
31 & Immune/\allowbreak{}Inflammatory & Lymphocyte & CD4 T cell & CD4, CD3E, IL7R & CCR7, LEF1 & \cite{pmid42056516,pmid41986723,pmid41951740} \\
32 & Immune/\allowbreak{}Inflammatory & Lymphocyte & Regulatory T cell & FOXP3, IL2RA, CTLA4 & IKZF2, TNFRSF18 & \cite{pmid41448182,pmid41932343,pmid38181095} \\
33 & Immune/\allowbreak{}Inflammatory & Lymphocyte & Gamma delta T cell & TRDC, TRGC1 & -- & \cite{pmid39058036,pmid42162424,pmid41708854} \\
34 & Immune/\allowbreak{}Inflammatory & Lymphocyte & NKT cell & CD3E, NCAM1, KLRB1 & -- & \cite{pmid39983726,pmid42190649} \\
35 & Immune/\allowbreak{}Inflammatory & Lymphocyte & B cell & CD19, CD20, MS4A1 & PAX5, CD79A & \cite{pmid42129565,pmid42056516,pmid42242231} \\
36 & Immune/\allowbreak{}Inflammatory & Plasma cell & Plasma cell & SDC1 (CD138), MZB1, JCHAIN & XBP1, PRDM1 & \cite{pmid42056516,pmid41593194,pmid40945518} \\
37 & Immune/\allowbreak{}Inflammatory & Macrophage/\allowbreak{}Histiocyte & Macrophage & CD68, CD163, CSF1R & MRC1, MARCO, MSR1 & \cite{pmid33357445,pmid41576929,pmid40345189} \\
38 & Immune/\allowbreak{}Inflammatory & Macrophage/\allowbreak{}Histiocyte & M1 macrophage & CD68, NOS2, TNF & IL1B, CXCL10, IDO1 & \cite{pmid42185888,pmid42049035,pmid33357445} \\
39 & Immune/\allowbreak{}Inflammatory & Macrophage/\allowbreak{}Histiocyte & M2 macrophage & CD68, CD163, MRC1 & TGFB1, IL10, ARG1 & \cite{pmid42056516,pmid41576929} \\
40 & Immune/\allowbreak{}Inflammatory & Macrophage/\allowbreak{}Histiocyte & Monocyte & CD14, LYZ, VCAN & -- & \cite{pmid41435820,pmid42030954,pmid40957419} \\
41 & Immune/\allowbreak{}Inflammatory & Macrophage/\allowbreak{}Histiocyte & Kupffer cell & CD68, CLEC4F, MARCO & -- & \cite{pmid42151416,pmid41131393} \\
42 & Immune/\allowbreak{}Inflammatory & Macrophage/\allowbreak{}Histiocyte & Alveolar macrophage & MARCO, FABP4, CD68 & -- & \cite{pmid41966692,pmid42208526,pmid42151416} \\
43 & Immune/\allowbreak{}Inflammatory & Macrophage/\allowbreak{}Histiocyte & Microglia & AIF1 (IBA1), CX3CR1, P2RY12 & TMEM119, TREM2 & \cite{pmid42020743,pmid42243549,pmid41576930} \\
44 & Immune/\allowbreak{}Inflammatory & Macrophage/\allowbreak{}Histiocyte & Osteoclast & ACP5, CTSK, MMP9 & -- & \cite{pmid38714197,pmid41592325,pmid41951740} \\
45 & Immune/\allowbreak{}Inflammatory & Other inflammatory & Dendritic cell & ITGAX, CD1C, CLEC9A & BATF3, IRF8 & \cite{pmid42154581,pmid42086564,pmid42218150} \\
46 & Immune/\allowbreak{}Inflammatory & Other inflammatory & Plasmacytoid DC & LILRA4, TCF4, IRF7 & -- & \cite{pmid42218150,pmid42020427} \\
47 & Immune/\allowbreak{}Inflammatory & Neutrophil & Neutrophil & ELANE, MPO, FCGR3B & CSF3R, CXCR2, S100A8 & \cite{pmid41576930,pmid42236943,pmid42203883} \\
48 & Immune/\allowbreak{}Inflammatory & Other inflammatory & Eosinophil & CLC, EPX, PRG2 & IL5RA, CCR3 & \cite{pmid42129565,pmid41990751,pmid42243549} \\
49 & Immune/\allowbreak{}Inflammatory & Other inflammatory & Mast cell & KIT, TPSAB1, CMA1 & FCER1A, HDC & \cite{pmid42056516,pmid42151416,pmid41992007} \\
50 & Immune/\allowbreak{}Inflammatory & Other inflammatory & Basophil & GATA2, HDC, CPA3 & -- & \cite{pmid39058036,pmid42020427} \\
51 & Immune/\allowbreak{}Inflammatory & Lymphocyte & NK cell & NCAM1, NKG7, GNLY & KLRD1, KLRB1, PRF1 & \cite{pmid42127218,pmid41791380,pmid42208526} \\
52 & Stromal/\allowbreak{}Structural & Fibroblast/\allowbreak{}Stromal cell & Fibroblast & VIM, COL1A1, DCN & LUM, COL3A1, PDGFRA & \cite{pmid39729995,pmid42204317,pmid41895277} \\
53 & Stromal/\allowbreak{}Structural & Fibroblast/\allowbreak{}Stromal cell & Myofibroblast & ACTA2, TAGLN, MYH11 & -- & \cite{pmid41895277,pmid41776110,pmid42127218} \\
54 & Stromal/\allowbreak{}Structural & Fibroblast/\allowbreak{}Stromal cell & Cancer associated fibroblast & FAP, PDPN, POSTN & TNC, MMP2, MMP11 & \cite{pmid42236943,pmid33357445,pmid41005303} \\
55 & Stromal/\allowbreak{}Structural & Fibroblast/\allowbreak{}Stromal cell & MyCAF & ACTA2, FAP, TAGLN & MYL9, CNN1 & \cite{pmid33357445,pmid42010061,pmid41781391} \\
56 & Stromal/\allowbreak{}Structural & Fibroblast/\allowbreak{}Stromal cell & ICAF & IL6, CXCL12, PDGFRA & CFD, DPT, HAS1 & \cite{pmid33357445,pmid41448182,pmid42010061} \\
57 & Stromal/\allowbreak{}Structural & Fibroblast/\allowbreak{}Stromal cell & ApCAF & CD74, HLA-DRA, SLPI & SAA1, SAA2 & \cite{pmid41005303,pmid41448182,pmid42010061} \\
58 & Stromal/\allowbreak{}Structural & Endothelial/\allowbreak{}Vessel-associated & Endothelial cell & PECAM1, VWF, CDH5 & FLT1, KDR, ERG & \cite{pmid41781666,pmid42091869,pmid42208495} \\
59 & Stromal/\allowbreak{}Structural & Endothelial/\allowbreak{}Vessel-associated & Lymphatic endothelial & LYVE1, PROX1, PDPN & FLT4, CCL21 & \cite{pmid41856521,pmid41986723,pmid41616773} \\
60 & Stromal/\allowbreak{}Structural & Endothelial/\allowbreak{}Vessel-associated & Tip cell & ESM1, APLN, DLL4 & -- & \cite{pmid42154581,pmid42126225} \\
61 & Stromal/\allowbreak{}Structural & Endothelial/\allowbreak{}Vessel-associated & Pericyte & RGS5, PDGFRB, NOTCH3 & MCAM, CSPG4 & \cite{pmid41529665,pmid40680742,pmid42208526} \\
62 & Stromal/\allowbreak{}Structural & Smooth muscle/\allowbreak{}Muscle & Smooth muscle cell & ACTA2, DES, MYH11 & CNN1, TAGLN, MYLK & \cite{pmid41895277,pmid42206386,pmid42236958} \\
63 & Stromal/\allowbreak{}Structural & Fibroblast/\allowbreak{}Stromal cell & Stellate cell & LRAT, PDGFRB, ACTA2 & -- & \cite{pmid42151416,pmid41238915,pmid41997362} \\
64 & Stromal/\allowbreak{}Structural & Fibroblast/\allowbreak{}Stromal cell & Mesothelial cell & MSLN, WT1, KRT5 & -- & \cite{pmid41005303,pmid42151416,pmid42056464} \\
65 & Stromal/\allowbreak{}Structural & Adipocyte/\allowbreak{}Fat & Adipocyte & ADIPOQ, LEP, FABP4 & PPARG, PLIN1 & \cite{pmid41534526,pmid41997362,pmid42056516} \\
66 & Stromal/\allowbreak{}Structural & Peripheral nerve/\allowbreak{}Schwann-associated & Schwann cell & S100B, SOX10, MPZ & -- & \cite{pmid41508044,pmid41512873,pmid41643676} \\
67 & Other/\allowbreak{}QC & Uncertain/\allowbreak{}low-confidence/\allowbreak{}non-evaluable & Erythrocyte & HBA1, HBB, HBA2 & SLC4A1, GYPA & \cite{pmid41703319,pmid38714197,pmid39567784} \\
68 & Other/\allowbreak{}QC & Uncertain/\allowbreak{}low-confidence/\allowbreak{}non-evaluable & Platelet megakaryocyte & ITGA2B, GP1BA, PF4 & -- & \cite{pmid41592325,pmid41703319,pmid41951740} \\
\end{longtable}
\endgroup
\clearpage
