# Supplementary material for: CellPath-Bench: A Multidimensional Benchmark for Whole-Slide Cellular Representations in Pathology Foundation Models
Source: arXiv:2608.21060 source file (2026-08-21)
Supplement: Supplementary file 3 [file cross_results_preamble.tex]

% CellPath-Bench — packages required by the cross-section result tables.
% Identical to the IS set; input either one, not both.
\usepackage{booktabs}
\usepackage{array}
\usepackage{float}
