# Supplementary material for: CellPath-Bench: A Multidimensional Benchmark for Whole-Slide Cellular Representations in Pathology Foundation Models
Source: arXiv:2608.21060 source file (2026-08-21)
Supplement: Supplementary file 4 [file is_results_preamble.tex]

% CellPath-Bench — packages required by the IS result tables.
%
% Input before \begin{document} in supplementary.tex, unless the main document
% already provides these.
%
% The tables are portrait and stretched to \textwidth, so neither rotating nor
% graphicx is needed, and there is no \resizebox anywhere. caption and subcaption
% are deliberately NOT loaded: they conflict with the AAAI template.
% float supplies the [H] specifier, which pins every table to the exact point
% where it is inputted, so no table can drift out of the section that contains it.
% threeparttable is no longer needed: the tables carry no note.
% None of these is on the AAAI forbidden-package list.

\usepackage{booktabs}
\usepackage{array}
\usepackage{float}
